# Supplementary material for: Generation of subcycle isolated attosecond pulses by pumping ionizing gating
Source: arXiv:2212.06599 source file (2023-07-30)
Supplement: Supplementary file 1 [file Supplement_material_of__Generation_of_subcycle_isolated_attosecond_pulses_by_pumping_ionizing_gating___0627__-2.pdf]

# Supplement material of "Generation of subcycle isolated attosecond pulses by pumping ionizing gating"

Zhaohui Wu,[1] Hao Peng,[2] Xiaoming Zeng,[1] Zhaoli Li,[1] Zhimeng Zhang,[1] Huabao Cao,[3] Yuxi Fu,[3] Xiaodong Wang,[4] Xiao Wang,[4] Jie Mu,[4] Yanlei Zuo,[4] C. Riconda,[4] S. Weber,[5] and Jingqin Su[1]
[1)] *Science and Technology on Plasma Physics Laboratory, Research Center of Laser Fusion, China Academy of Engineering Physics, Mianyang, Sichuan, China, 621900.*
[2)] *College of Physics and Optoelectronic Engineering, Shenzhen University, Shenzhen 518060, China*
[3)] *Center for Attosecond Science and Technology, State Key Laboratory of Transient Optics and Photonics, Xi'an Institute of Optics and Precision Mechanics, Chinese Academy of Sciences, Xi'an 710119, Shaanxi, China*
[4)] *LULI, Sorbonne Université, CNRS, École Polytechnique, CEA, F-75005, Pari, France*
[5)] *ELI Beamlines facility, Extreme Light Infrastructure ERIC, 25241 Dolni Brezany, Czech Republic*

## I. ANALYTICAL SOLUTION

In order to understand the physical mechanism behind the pumping ionizing gating (PIG) process, we begin by examining the energy transfer from the pump pulse to the driving pulse via a fast-extending plasma grating (FEPG). This process can be described using the three-waves coupling equations for laser-plasma interaction[1]:

$$\begin{aligned}
&(\tfrac{\partial^2}{\partial t^2} - c^2\Delta^2 + \omega_{pe}^2)\mathbf{A} = -\tfrac{4\pi e^2}{m_e}\delta n_e \mathbf{A}_0,\\
&(\tfrac{\partial^2}{\partial t^2} - c^2\Delta^2 + \omega_{pe}^2)\mathbf{A}_0 = -\tfrac{4\pi e^2}{m_e}\delta n_e \mathbf{A},\\
&(\tfrac{\partial^2}{\partial t^2} - c_s^2\Delta^2)\delta n_e = \tfrac{Ze^2 n_{e0}}{m_e m_i c^2}\Delta^2(\mathbf{A}\mathbf{A}_0),
\end{aligned} \tag{1}$$

where $\mathbf{A}_0$ and $\mathbf{A}$ are laser vector potentials of the pump and the driving pulse, respectively, $c_s = \sqrt{ZT_e/m_i}$ is the ion acoustic velocity, $Z$ is the plasma ion charge, $T_e$ is the plasma temperature, $e$ is the electron charge, $m_{e(i)}$ is the electron(ion) mass, $\delta n_e$ is the amplitude of electron density perturbation, and $n_{e0}$ is the average electron density.

The laser electric field is $\mathbf{E} = -\frac{1}{c}\frac{\partial \mathbf{A}}{\partial t}$, and the 1-dimensional(1D) electric field can be written $\mathbf{E}_0 = \frac{1}{2}E_0 exp[-i(\omega_0 t - k_0 x) + c.c.]$ and $\mathbf{E} = \frac{1}{2}E exp[-i(\omega t + kx) + c.c.]$, where $\omega_0$ and $k_0$ are the pump frequency and wave number, $\omega$ and $k$ are the frequency and wave number of the driving pulse, respectively. By using the slowly-varying envelope approximation, the Eq.1 can be simplified to[1]:

$$\begin{aligned}
&\tfrac{\partial E_0}{\partial t} - v_g \tfrac{\partial E_0}{\partial z} = -i\tfrac{\omega_{pe}^2}{2\omega_0}E f^*,\\
&\tfrac{\partial E}{\partial t} + v_g \tfrac{\partial E}{\partial z} = -i\tfrac{\omega_{pe}^2}{2\omega_0}E f,\\
&(\tfrac{\partial^2}{\partial t} - c_s^2\tfrac{\partial^2}{\partial z^2})f = \tfrac{Ze^2}{4m_e m_i c^2}E_0 E^*,
\end{aligned} \tag{2}$$

where $\omega_{pe} = \sqrt{4\pi n_e e^2/m_e}$ is the plasma frequency, $f \equiv \frac{\delta n_{e0}}{n_{e0}}$ is the normalized plasma density, $k_B$ and $\omega_B$ are the wave number and frequency of the ion acoustic wave.

In the limit of a low pump intensity below the ionization threshold and temporal scale of attosecond, the influence of plasma grating from laser pulses can be neglected. Therefore, in the variable of $\xi = z - v_g t$, Eq.2 can be written as[2]

$$\begin{aligned}
&\tfrac{\partial E}{\partial_t} = -i\tfrac{\omega_{pe}^2}{2\omega_0}E_0 f e^{2i\omega_0 \delta N t},\\
&\tfrac{\partial E_0}{\partial_t} + 2v_g\tfrac{\partial E_0}{\partial \xi} = -i\tfrac{\omega_{pe}^2}{2\omega_0}E f e^{-2i\omega_0 \delta N t},
\end{aligned} \tag{3}$$

where $\delta N$ is the difference of refractive index between the point $\xi$ and the resonant point $\xi_0$.

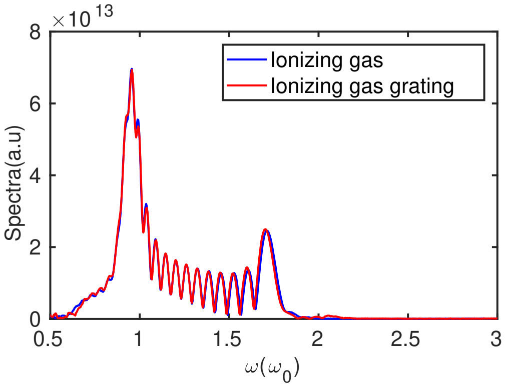


FIG. S1. PIC simulation of the laser spectra in the ionizing gas and gas grating at $t = 200\lambda_0/c$. The laser has a FWHM duration of 30 fs, a peak intensity of $10^{15}$ W/cm$^2$ and central wavelength of $\lambda_0 = 1$ $\mu$m. Both the background gas and gas grating have an average density of $0.1n_c$. The gas grating has a period of $\Lambda \geq 0.8\lambda_0$ or $\lambda \leq 0.3\lambda_0$, and a modulation depth of $0.05n_c$.

In a medium with a time-varying refractive index, the laser experiences a frequency shift while maintaining a constant wavevector in order to satisfy the dispersion relation[3]. Theoretical models have been developed to describe this phenomenon in ionizing plasma[4–6]. In the case of the gradient plasma grating, although the periodic structure also provides a time-varying refractive index, the integration over one period is close to zero. Consequently, the frequency upconversion effect resulting from the periodic structure can be neglected, allowing us to extend the existing theoretical models for the gradient FEPG. To validate this assumption, we conducted

particle-in-cell (PIC) simulations using the same laser pulse to ionize the gas and the gas grating. In the simulation, the grating period is set as $\Lambda \geq 0.8\lambda_0$ or $\Lambda \leq 0.3\lambda_0$ in case that the laser is reflected by the plasma grating, so both the laser pulses in the gas and gas grating can keep the same. The spectra were found to be nearly identical, as shown in FigS1, implying the upconversion effect is not impacted by the periodic structure of the plasma grating.

In variable $\xi = z - v_g t$, the up-converted light can be presented as[3]

$$(\frac{2}{v_g}\frac{\partial}{\partial \xi} - \frac{1}{{v_g}^2}\frac{\partial}{\partial t})\frac{\partial}{\partial t}\mathbf{E} = \frac{\omega_{pe}}{{v_g}^2}\frac{n_e}{n_{e0}}\mathbf{E}. \quad (4)$$

In general, the IAP can be obtained by numerically solving Eq.3 and Eq.4. In the limit of a linear plasma gradient and $\omega_{pe} \ll \omega$, the second-order t derivative in Eq.4 can be neglected. Assuming the initial electric field is $\mathbf{E} = Eexp(i\omega/\xi)$, Eq.4 has an analytical solution of $\frac{\omega_0}{\omega}Ee^{i\omega t(\xi-\xi_0)}$ at $-L < \xi < 0$, where $\omega = \omega_0(1+ct\omega_{pe}^2/L\omega_0^2)^{1/2}$ is the shifted laser frequency,[3].

For a laser induced plasma, a roughly linear density gradient can be formed in the pulse front. The up-converted light has an analytical solution of $\frac{\omega_0}{\omega}Ee^{i\omega t(\xi-\xi_0)}$ when $\omega_{pe} \ll \omega$, where $\omega = \omega_0(1 + ct\omega_{pe}^2/L\omega_0^2)^{1/2}$ is the shifted laser frequency[3]. However, the up-converted process in PIG more complex due the reflected pump. As the reflected pump is mainly affected by the plasma gradient and the propagation time, it can be approximately divided into a series of independent infinitesimal pulses. For $dE$ at time $t$, the up-converted electric field at time $t + \delta t$ can be described by Eq.5.

$$dE(t + \delta t) = \frac{\omega_0}{\omega_0(\delta t)}dEe^{i\omega(\delta t)(\xi-\xi_0)}. \quad (5)$$

As the resonant region in gradient FPEG is very narrow, the pump reflectivity is small and $E_0$ is approximated to a constant in Eq.3, so it is

$$dE = -i\frac{\omega_{pe}^2}{2\omega_0}E_0 f e^{2i\omega_0\delta N t}dt. \quad (6)$$

Combing Eq.6 with Eq.5, the IAP has the following analytical solution

$$E = \int_0^t i\frac{\omega_{pe}^2}{2\omega}E_0 f e^{2i\omega_0\delta N t + i\omega(\xi-\xi_0)}dt. \quad (7)$$

## II. PIC SIMULATION

The details of the simulation results with varying average densities and modulation depths are displayed in Fig.S2. As shown in Fig.S2(a) and Fig.S2(c), for $n_{e0}$ from $0.02n_c$ to $0.5n_c$, the Full Width at Half Maximum (FWHM) pulse duration is found to gradually decrease as the interaction length increases, reaching sub-500 attoseconds. After that, it does not further decrease but oscillates between $\sim$ 1fs and hundred of attoseconds. The oscillation has a period about hundreds of femtosecond,

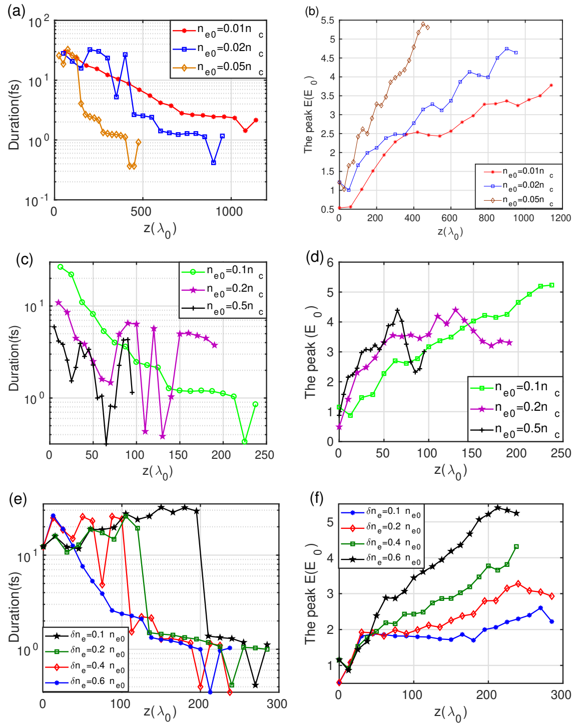


FIG. S2. 1D simulation of IAP generation at various plasma densities and FEPG modulation depths. Evolution of (a,c) the FWHM duration and (b,d) electric field of the driving pulse $E$ at average plasma densities from $0.01n_c$ to $0.5n_c$. Evolution of the FWHM duration(e) and $E$ at different FEPG modulation depths.

implying that it is mainly due to the plasma instabilities such as the fluctuations of the plasma density with a similar oscillation period, which makes the pump reflection not exactly overlap with the IAP peak when the pulse duration is too short. In the experiment, a proper interaction length can be set by adjusting the pump focal depth or the length of gas gratings. The required interaction length for IAP decreases with higher plasma density, attributed to a stronger upconversion effect at higher densities. The peak electric field of the driving pulse initially increases with plasma density, reaching a maximum value between $4E_0$ and $6E_0$ before saturating, as shown in Fig.S2(b) and Fig.S2(d). The conversion efficiency increased from 0.14% to 1.3% as the plasma density increased from $0.02n_c$ to $0.5n_c$. However, for plasma densities above $0.1n_c$, both the electric field and pulse duration became unstable due to more serious plasma instabilities such as modulation instability[2,7] and group velocity dispersion, as shown in Fig.S2(c). Based on these results, a plasma density of $0.1n_c$ was determined to be optimal for the IAP generation in the simulation. Moreover, for $n_{e0} = 0.1n_c$, the simulation results with the FEPG amplitudes from $60\%n_{e0}$ to $10\%n_{e0}$ are displayed in Fig.S2(e)-(f). The simulation results show that the peak electric field of the driving pulse decreases as the FEPG modulation depth decreases, and the required

length of the plasma increases accordingly. However, the shortest pulse duration is little affected, and sub-500-attoseconds pulses can still be obtained at $\delta n_e = 10\% n_{e0}$. This suggests that the generation of IAPs is not strongly dependent on a large FEPG amplitude.

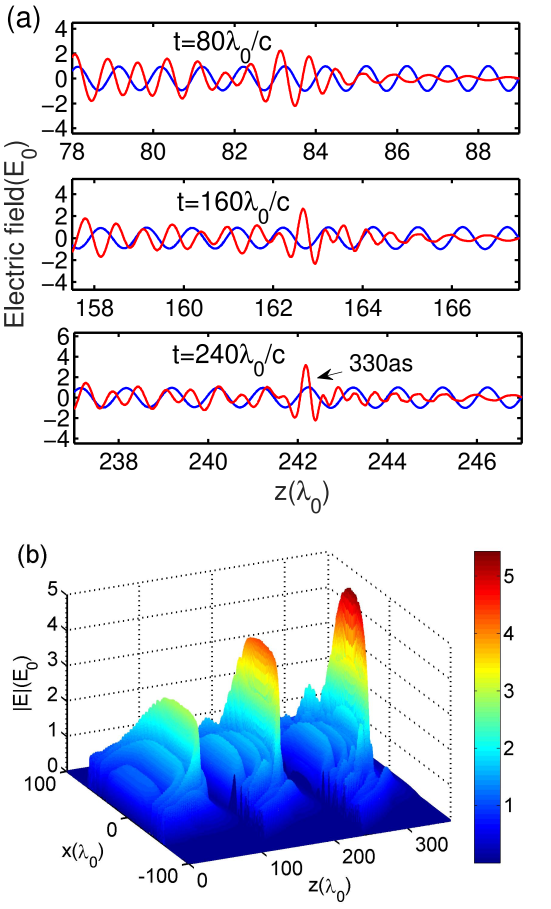


FIG. S3. (a)1D waveforms of the driving pulse(red curves) and the pump(blue curves) at different interaction time.(b) 2D electric field of the driving pulse at different interaction time.

TABLE S1. Optimal parameters for the simulation of IAPs, where $\lambda$, $I$, $\tau$ and $R$ are the laser central wavelength, peak intensity, FWHM duration and beam waist, respectively, $L_i$ is the length of gas grating.

| Pump | $\lambda(\mu m)$ | $I(W/cm^2)$ | $\tau(ps)$ | R($\mu m$) |
|---|---|---|---|---|
| Value | 1 | $4 \times 10^{13}$ | 1.6 | 50 |
| Driving pulse | $\lambda(\mu m)$ | $I(W/cm^2)$ | $\tau(fs)$ | R($\mu m$) |
| value | Arbitrary | $1 \times 10^{14}$ | 30 | 50 |
| Gas grating | $n_{e0}(n_c)$ | $\delta n_{e0}/n_{e0}$ | $\Lambda(\mu m)$ | $L_i(\mu m)$ |
| Value | 0.1 | 0.5 | 0.507 | 240 |

The summary of the optimal parameter is given in Tab.S1, with which the 1D to 3D simulation results of IAP evolution are conducted. As the 3D simulation result is given in the main text, the 1D and 2D simulation results are supplemented here. The 1D simulation used a cell size of $\Delta z = \lambda_0/200$, and we found that decreasing the cell size to $\lambda_0/1000$ did not significantly affect the results, indicating that this cell size is sufficient for accurately simulating the IAP generation. The waveforms of the driving pulse and pump at different times are shown in Fig.S3(a). The amplitude of the driving pulse gradually increases to about $5.75E_0$ while the pulse duration decreases to 330 as. The pump waveform remains almost the same as it passes through the FEPG, implying a low reflectivity. In the 2D simulation, the cell size was set to $\Delta x \times \Delta z = \lambda_0/10 \times \lambda_0/200$, with $x$ and $z$ representing the transverse and longitudinal directions, respectively. As shown in Fig.S3(b), while the beam size of the driving pulse tends to decrease as it grows, it maintains a high level of uniformity and quality.

A video named 1Dsimulation.avi is provided to show the dynamically process of how the IAP is formed in the 1D simulation. In the video, the green fringes are the background gas grating while the dark green fringes are the ionized plasma grating, the blue pulse is the pump, and the red pulse driving pulse.

[1] W. L. Kruer, *The Physics of Laser Plasma Interaction* (Addison-Wesley, New York, 1988).

[2] Z. Wu, X. Zeng, Z. Li, Z. Zhang, X. Wang, B. Hu, X. Wang, J. Mu, J. Su, Q. Zhu, X. Wei, , and Y. Zuo, Matter Radiate Extreme **7**, 064402 (2022).

[3] E. Esarey, G. Joyce, and P. Sprangle, Phys. Rev. A **44**, 3908 (1991).

[4] K. Qu, Q. Jia, M. R. Edwards, and N. J. Fisch, Phys. Rev. E **98**, 023202 (2018).

[5] K.Qu and N. Fisch, Phys. Rev. E **99**, 063201 (2019).

[6] A. J. Howard, D. Turnbull, A. S. Davies, P. Franke, D. H. Froula, , and J. P. Palastro, Phys. Rev. Lett. **123**, 124801 (2019).

[7] V. M. Malkin, G. Shvets, and N. J. Fisch, Phys. Rev. Lett **82**, 4448 (1999).
